# Supplementary material for: Convergence of diffusions and their discretizations: from continuous to discrete processes and back
Source: arXiv:1904.09808 source file (2020-05-01)
Supplement: Supplementary file 1 [file intro_supp.tex]

\section{Introduction}

In this supplement of \cite{debortoli2019back} we present the proofs of
\cite[\Cref{sec:presentation}]{debortoli2019back} in
\Cref{sec:presentation_proof}, \cite[\Cref{sec:applications}]{debortoli2019back}
in \Cref{sec:applications:proof} and
\cite[\Cref{sec:quant-conv-bounds}]{debortoli2019back} in
\Cref{sec:quant-conv-bounds:proof}.  We present a minorization condition for
functional autoregressive models, which is a generalization of \cite[Section
6]{durmus:moulines:2016} in \Cref{sec:mino_condition_AR}. We also derive in
\Cref{sec:quant-conv-results} the proof of a general convergence result for
Markov coupling kernels which mainly borrow from \cite[Lemma
19.4.2]{douc:moulines:priouret:soulier:2018}.  An application of the results of
\cite[\Cref{sec:main-results00}]{debortoli2019back} to the case of the tamed
Euler-Maruyama discretization of a diffusion is presented in
\Cref{sec:tamed-unadj-lang}.  Explicit rates and a discussion on the dependency
of the bounds identified in the convergence of the projected Euler-Maruyama in
$V$-norm under weak curvature conditions is discussed in
\Cref{sec:rates-crefpr}.

%%% Local Variables:
%%% mode: latex
%%% TeX-master: "supplementary"
%%% End:
